# Supplementary material for: Video-Bench: Human-Aligned Video Generation Benchmark
Source: arXiv:2504.04907 source file (2025-04-29)
Supplement: Supplementary file 1 [file main_supp.tex]

% CVPR 2025 Paper Template; see https://github.com/cvpr-org/author-kit

\documentclass[10pt,twocolumn,letterpaper]{article}

%%%%%%%%% PAPER TYPE  - PLEASE UPDATE FOR FINAL VERSION
\usepackage{cvpr}              % To produce the CAMERA-READY version
\usepackage{multirow}
% Import additional packages in the preamble file, before hyperref

\usepackage{pifont}
\usepackage{graphicx}  % 引入graphicx包以使用\scalebox
\usepackage{listings}
\usepackage{subcaption}   % 控制子表格
\usepackage{cuted}
\usepackage{float}
% strip environment
\usepackage{caption}    % For better caption control
\usepackage{soul}
\usepackage{xcolor}
\usepackage{pifont}
\usepackage{tikz}
\usepackage[utf8]{inputenc}
\usepackage{tcolorbox}
\usepackage{xcolor}
\usepackage{pifont}
\usepackage{geometry}
\usepackage{amsmath} % 用于数学符号
\usepackage{amssymb} % 用于符号如 \dag
\geometry{a4paper, margin=1in}

\usepackage{hyperref}

\usepackage{minted}
\usemintedstyle{default}  % 选择默认的代码高亮风格
\usemintedstyle{default}  % 选择默认的代码高亮风格
\setminted{
  fontsize=\scriptsize,  % 代码字体大小
  baselinestretch=1.1,  % 行距
  breaklines=true,  % 自动换行
  framesep=2mm,  % 代码与边框的距离（可以留作内边距）
  tabsize=2,  % Tab键的空格大小
  bgcolor=gray!10,  % 设置背景颜色为浅灰色
}

\definecolor{customgreen}{rgb}{0.35, 0.65, 0.35}
\definecolor{customred}{rgb}{0.7, 0.35, 0.35}
\definecolor{customblue}{rgb}{0.3, 0.6, 0.8}
\definecolor{customblue1}{rgb}{0.3, 0.6, 0.8}
\definecolor{customblack}{rgb}{0.2, 0.2, 0.2}

% 定义一个新命令来创建黑色圆圈白色数字

 % 定义绿色对勾
   % 定义红色叉号

\definecolor{darkred}{rgb}{0.6, 0, 0}
\definecolor{darkgreen}{rgb}{0, 0.5, 0}
\definecolor{darkblue}{rgb}{0, 0, 0.55}
\input{preamble}

% It is strongly recommended to use hyperref, especially for the review version.
% hyperref with option pagebackref eases the reviewers' job.
% Please disable hyperref *only* if you encounter grave issues, 
% e.g. with the file validation for the camera-ready version.
%
% If you comment hyperref and then uncomment it, you should delete *.aux before re-running LaTeX.
% (Or just hit 'q' on the first LaTeX run, let it finish, and you should be clear).
\definecolor{cvprblue}{rgb}{0.21,0.49,0.74}
%\usepackage[pagebackref,breaklinks,colorlinks,allcolors=cvprblue]{hyperref}

%%%%%%%%% PAPER ID  - PLEASE UPDATE
 % *** Enter the Paper ID here

%%%%%%%%% TITLE - PLEASE UPDATE
% \title{
% \textit{Supplementary Material:} {HA-Video-Bench}: \underline{H}uman Preference \\\underline{A}ligned \underline{Video} Generation \underline{Bench}mark
% }

\title{
Video-Bench: Human-Aligned Video Generation Benchmark
}

% 自定义符号顺序
\renewcommand{\fnsymbol}[1]{%
  \ifcase#1\relax
    † % 第一个符号是 †
  \or
    * % 第二个符号是 *
  \else
    \fnsymbol{#1} % 其他符号使用默认顺序
  \fi
}

\author{
    Hui Han$^{1}$\thanks{Equal Contribution.}\footnotemark[1] \hspace{1cm} 
    Siyuan Li$^{1}$\footnotemark[1] \hspace{1cm}
    Jiaqi Chen$^{2,3}$\footnotemark[1] \hspace{1cm} 
    Yiwen Yuan$^{4}$\footnotemark[1] \\
    Yuling Wu$^4$ \hspace{0.6cm} 
    Chak Tou Leong$^5$ \hspace{0.6cm} 
    Hanwen Du$^6$ \hspace{0.6cm} 
    Junchen Fu$^7$ \hspace{0.6cm} 
    Youhua Li$^8$ \hspace{1cm} \\
    Jie Zhang$^2$ \hspace{1cm} 
    Chi Zhang$^{9}$ \hspace{1cm} 
    Li-jia Li$^{10}$ \hspace{1cm} 
    Yongxin Ni$^{11}$\thanks{Corresponding author (email: niyongxin@u.nus.edu).}
        \vspace{.5em}
    \\
    $^1$Shanghai Jiao Tong University 
    \quad
    $^2$Fudan University 
    \quad
    $^3$Stanford University 
    \quad \\
    $^4$Carnegie Mellon University 
    \quad
    $^5$Hong Kong Polytechnic University
    \quad \\
    $^6$Soochow University
    \quad
    $^7$University of Glasgow
    \quad 
    $^8$City University of Hong Kong
    \quad \\
    $^{9}$Westlake University
    \quad
    $^{10}$LiveX AI
    \quad
    $^{11}$National University of Singapore
      \vspace{.5em} 
  \\
  \textcolor{black}{\url{https://github.com/Video-Bench/Video-Bench.git}}
}

\begin{document}

% \maketitle

% 手动添加符号说明
% \vspace{1em} % 增加垂直间距，使说明与作者列表分开
% \noindent
% \textsuperscript{\dag} Equal contribution. \\
% \textsuperscript{*} Corresponding author.
 
% \input{figure/dimension}
% \input{sec/0_abstract}    
% \input{sec/1_intro}
% \input{sec/2_related}
% \input{sec/3_benchmark}
% \input{sec/4_method}
% \input{sec/5_experiment}
% \input{sec/6_results}
% \input{sec/7_conclusion}

% \clearpage
\appendix

% \maketitlesupplementary
\input{sec/X_suppl}
{\small
\bibliographystyle{ieeenat_fullname}
\bibliography{cited}}
%%%%%%%%% REFERENCES

% WARNING: do not forget to delete the supplementary pages from your submission 

\end{document}
